# Supplementary material for: Understanding Deep Networks via Extremal Perturbations and Smooth Masks
Source: arXiv:1910.08485 source file (2019-10-18)
Supplement: Supplementary file 1 [file suppl.tex]

\section{Supplementray material}\label{s:suppl}

\begin{figure}
\centering
\includegraphics[width=0.8\linewidth]{area_loss.pdf}
\caption{\textbf{Area constraint.}
The blue line is the reference vector $\mathbf{r}_a$ representing the target area $a$ as a proportion of ``on'' versus ``off'' pixels (here $a=80\%$).
The red dotted lines represent mask values in ascending, sorted order, $\sortvec(\bbm)$, at different points of the optimization, staring by initializing $\bbm$ to $1/2$.
Over time, the optimization encourages the mask to match the target area.
Even in the limit, there is a slight difference between  $\mathbf{r}_a$ as $\bbm$ as the latter is forced to be smooth at the boundaries; this has the further beneficial effect of minimizing the boundary length, encouraging more compact masks.
}\label{fig:area_norm}
\end{figure}

\input{fig-maxconv-1d}
\begin{figure}
\centering
\includegraphics[width=\linewidth]{mask_generation.pdf}
\caption{\textbf{Generating smooth masks.}
a. We first define a low resolution parameterization mask, $\bar\bbm \in [0,1]^{H \times W}$ (shown as a binary mask in this illustration).
b. We then represent each location in $\bar \bbm$ as a high resolution, smooth Gaussian, weighted by the value in $\bar\bbm$.
c. Finally, we apply the smooth max operator $...$ across all locations to get our final mask.}\label{fig:mask_generation}
\end{figure}
\begin{figure}
\centering
\includegraphics[width=0.3\linewidth]{000025_class_cow_9.pdf}
\includegraphics[width=0.3\linewidth]{000058_class_person_14.pdf}
\includegraphics[width=0.3\linewidth]{000069_class_boat_3.pdf}
\includegraphics[width=0.3\linewidth]{000025_class_person_14.pdf}
\includegraphics[width=0.3\linewidth]{000058_class_motorbike_13.pdf}
\includegraphics[width=0.3\linewidth]{000069_class_person_14.pdf}
\caption{\textbf{Pointing Examples from PASCAL}. Here we see a few examples of where our method is able to localize well to different objects in the image. The overlaid visualization is the average mask after Gaussian smoothing ($\sigma = 20$).}\label{fig:pointing-examples}
\end{figure}

We can in fact formally \emph{compare} the explanation provided by the linearization and extremal perturbation as the following two statements about \emph{sets} of images:
\begin{align}
\forall \bx : |\bx' - \bx| < \delta
&\Rightarrow
\Big|
\Phi(\bx') - \langle \nabla \Phi(\bx), \bx' - \bx \rangle - \Phi(\bx)
\Big| < \epsilon,
\label{e:def_extremal}
\\
\forall \bbm : |\bbm| < a^*
&\Rightarrow
\Phi(\bbm \otimes \bx) < \Phi(\bx).
\end{align}
\begin{equation}
\forall \bbm : |\bbm| < a^*
&\Rightarrow
\Phi(\bbm \otimes \bx) < \Phi(\bx).
\end{equation}
